# Supplementary material for: Night-to-Day Translation via Illumination Degradation Disentanglement
Source: arXiv:2411.14504 source file (2024-11-21)
Supplement: Supplementary file 1 [file X_suppl.tex]

\clearpage
\setcounter{page}{1}
\maketitlesupplementary

\section{Proof of Corollary 1} \label{sec:1}
We provide a detailed proof process to demonstrate how the invariant $N_{{\lambda}^m x^n}$ is exclusively related to the illumination and can function as the light effect detector. First, consider the following equations:
\begin{equation} 
    \small
    \begin{gathered}
    \begin{aligned}
     & N_{{\lambda}^m x^n} = \frac{\partial^{m+n-2}}{\partial \lambda^{m-1}  \partial x^{n-1}} \frac{\partial}{\partial x} \{\frac{1}{E(\lambda, x)} \frac{\partial E(\lambda, x) }{\partial \lambda} \}\\   
      &= \frac{\partial^{m+n-2}}{\partial \lambda^{m-1}  \partial x^{n-1}} \frac{\partial}{\partial x} \{\frac{1}{e(\lambda, x)} \frac{\partial e(\lambda, x)}{\partial \lambda } +\frac{1}{R(\lambda)C(x)} \frac{\partial R(\lambda)C(x) }{\partial \lambda } \} , \\
   \end{aligned}
    \end{gathered}	
    \label{eq: N-1-supp}
\end{equation}
by applying the additivity of linear differential operators, the first term represents the invariants only related to the illumination. The second term can be simplified by applying the chain rule as follows:
\begin{equation} 
    \begin{aligned}
    \small
      &\frac{\partial}{\partial x} \{ \frac{1}{R(\lambda)C(x)} \frac{\partial R(\lambda)C(x) }{\partial \lambda } \}\\
       &=  \frac{1}{R(\lambda)^2C(x)^2} (\frac{\partial^2 \{R(\lambda)C(x)\} } {\partial \lambda \partial x } \cdot R(\lambda)C(x) \\
        &-  \frac{\partial \{R(\lambda)C(x) \} }{\partial \lambda} \cdot \frac{\partial \{ R(\lambda)C(x) \} }{ \partial x}) \\
      &=  \frac{1}{R(\lambda)^2C(x)^2} ( \frac{\partial R(\lambda)}{\partial \lambda}\frac{\partial C(x)}{\partial x} \cdot R(\lambda)C(x)  \\
       &- \frac{\partial R(\lambda)}{\partial \lambda} C(x) \cdot R(\lambda) \frac{\partial C(x)}{\partial x} ) \\
       &=  0.
    \end{aligned}	
    \label{eq: N-2-supp}
\end{equation}

Finally, we conclude that the invariant $N_{{\lambda}^m x^n}$ is \textbf{exclusively related to the illumination} and can be formulated as follows:
\begin{equation} 
    \begin{gathered}
    \begin{aligned}
      N_{{\lambda}^m x^n} &= \frac{\partial^{m+n-2}}{\partial \lambda^{m-1}  \partial x^{n-1}} \frac{\partial}{\partial x} \{\frac{1}{E(\lambda, x)} \frac{\partial E(\lambda, x) }{\partial \lambda} \}\\   
      &= \frac{\partial^{m+n-1}}{\partial \lambda^{m-1}  \partial x^n}  \{\frac{1}{e(\lambda, x)} \frac{\partial e(\lambda, x)}{\partial \lambda } \}.
      \end{aligned}
    \end{gathered}	
    \label{eq: N-3-supp}
\end{equation}

\section{Limitations and Failure Case} \label{sec:2}
Despite the superior performance of N2D3 in Night2Day, it still exhibits certain limitations. On the one hand, this work focuses solely on addressing light degradation, while nighttime environments encompass various other types of degradation, including blur caused by rain, motion, and other factors. Our method currently struggles to handle these situations effectively. On the other hand, the limitations of visible imaging in night vision arise from the scarcity of photos captured in low-light conditions, as illustrated by the failure cases presented in\cref{fig:failure case supp}. Future advancements in night vision will likely incorporate additional modalities, such as infrared images, radar, and other sensor data, to overcome these challenges and improve performance.

\section{Implementation Details} \label{sec:3}
\textbf{Training Details.}
We adopt the \textit{resnet\underline{\hspace{0.2cm}}9blocks}, a ResNetbased model with nine residual blocks, as the backbone for generator $G$. Additionally, we utilize the patch-wise discriminator $D$ following PatchGAN\cite{isola2017image}. To conduct degradation-aware contrastive learning on multiple layers, we extract features from 5 layers of the generator $G$ encoder, as done in \cite{park2020contrastive}. These layers include RGB pixels, the first and second downsampling convolution, and the first and fifth residual block. For the features of each layer, we apply a 2-layer MLP to acquire final 256-dimensional features. These features are then utilized in our degradation-aware contrastive learning.

All the comparison methods are reproduced using their released source code with default settings. Training procedures are consistent across all methods. All models are trained using the Adaptive Moment Estimation optimizer with an initial learning rate of $10^{-4}$, a momentum of 0.9, and weight decay of $10^{-4}$. For the BDD100K dataset, training consists of 10 epochs with the initial learning rate, followed by another 10 epochs with a decreased learning rate using the polynomial annealing procedure with a power of 0.9. On the Alderley dataset, given the limited training data compared to BDD100K, we extend the training to 20 epochs with the initial learning rate and an additional 20 epochs with the decayed learning rate. All the experiments are run on a single A100 GPU with 80GB of memory. Training our method with a smaller patch size and batch size on a device with less memory is feasible.

\textbf{Evaluation Details.}
In the evaluation, we compute the \emph{Fréchet Inception Distance} (FID) \cite{heusel2017gans}, Structural Similarity Index (SSIM) \cite{ssim}, and Learned Perceptual Image Patch Similarity (LPIPS) \cite{LPIPS} scores on $256\times512$ images. Partial FID scores are provided by ForkGAN \cite{zheng2020forkgan}, and all SSIM and LPIPS scores are reproduced by us.

Semantic segmentation evaluation are conducted as follows. First, we use Deeplabv3 pretrained on the Cityscapes dataset as the semantic segmentation model \cite{chen2017rethinking}. The model is provided by \url{https://github.com/open-mmlab/mmsegmentation} with an R-18-D8 backbone and trained at a resolution of $512\times1024$. Second, we perform $512\times1024$ Night2Day translation to obtain the generation results. Finally, we infer the semantic segmentation on the generated daytime images.

\begin{figure*}[t]
\centering
\includegraphics[width=0.99\linewidth]{./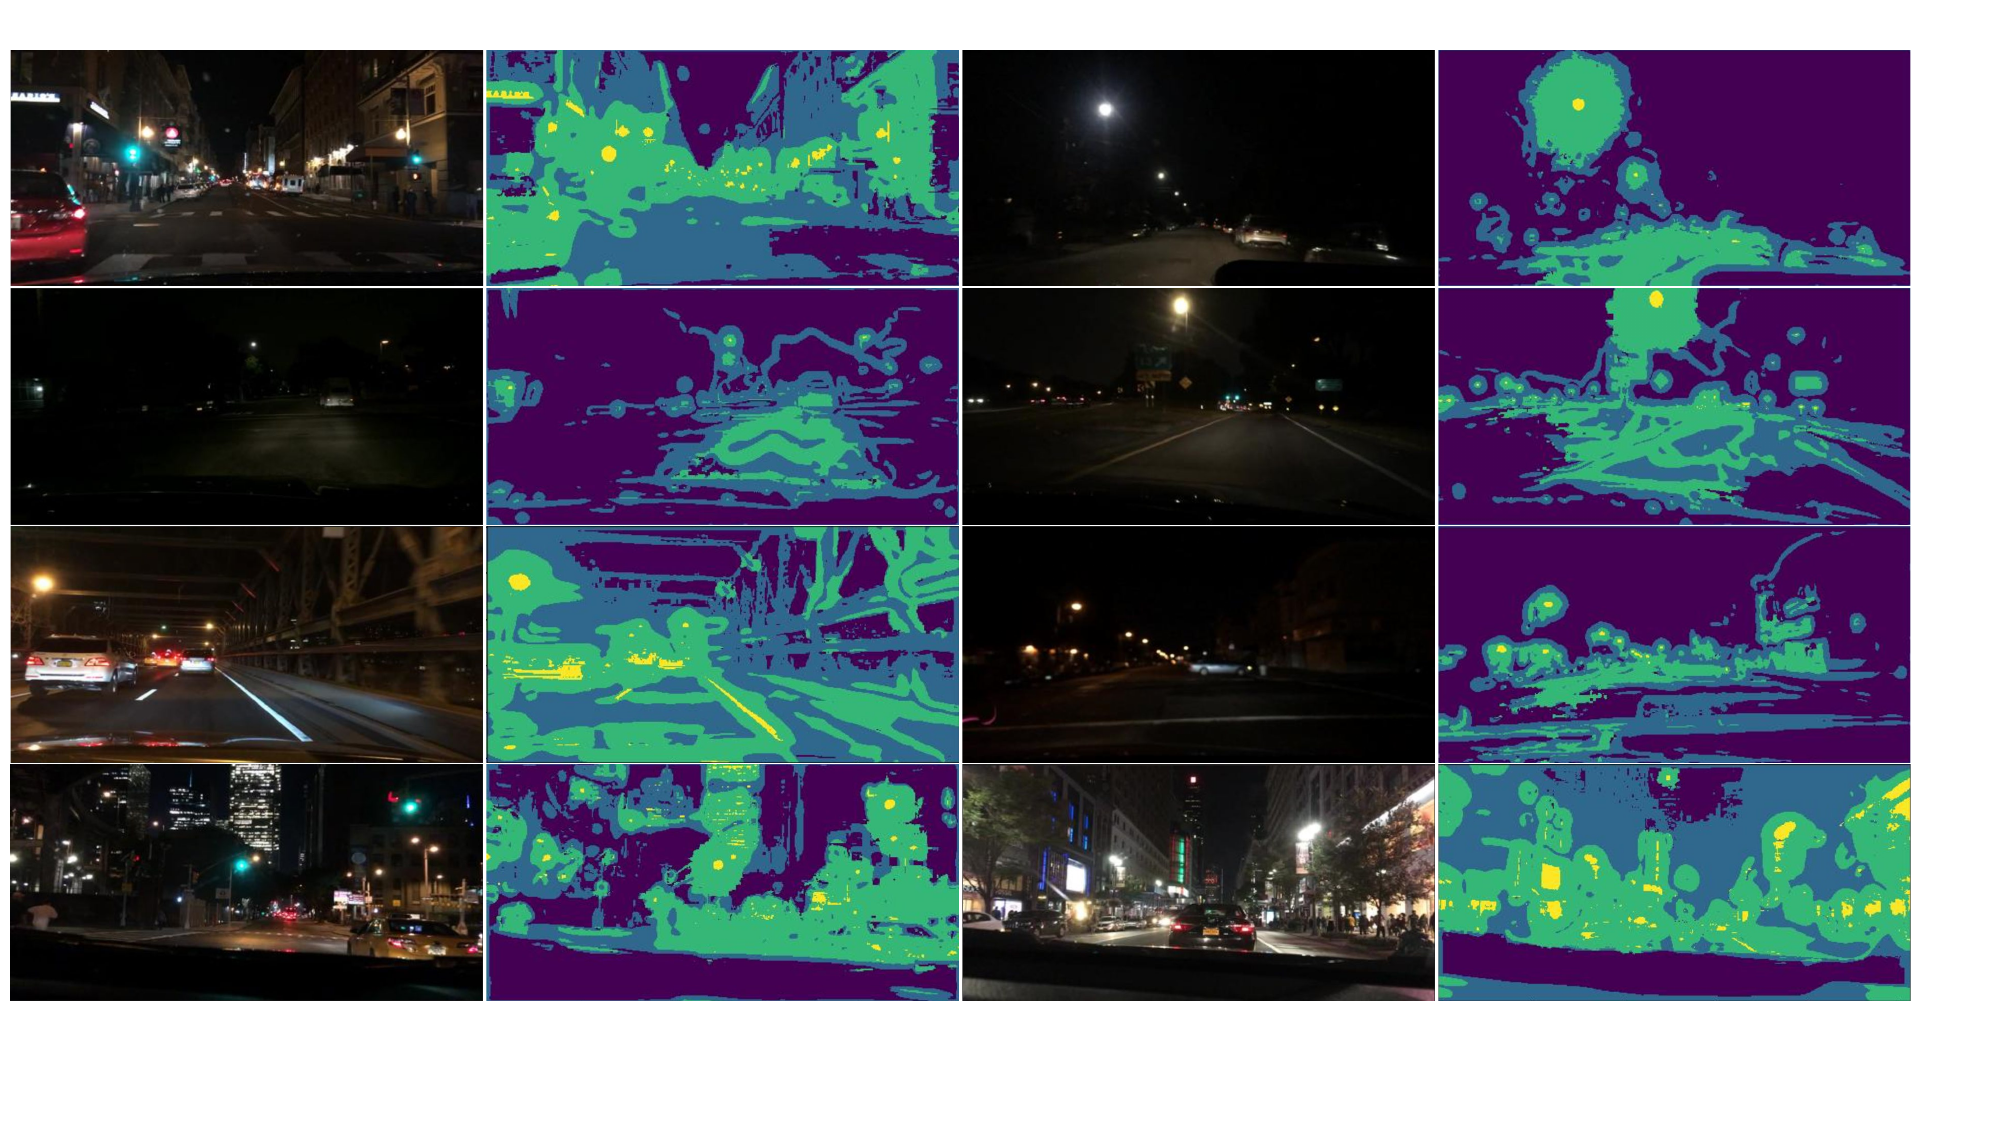} 
\vspace{-0.2cm}
\caption{More disentanglement results. The first and third rows display nighttime images, while the second and fourth rows show the corresponding degradation disentanglement results. The color progression from \textbf{\textcolor{blue}{blue}}, \textbf{\textcolor{blue!50}{light blue}}, \textbf{\textcolor{green!70}{green}} to \textbf{\textcolor{yellow!100}{yellow}} corresponds to the following regions: darkness, well-lit, light effects, and high-light.}
\vspace{-0.3cm}
\label{fig: dis results supp}
\end{figure*}

\begin{figure*}[t]
\centering
\includegraphics[width=0.99\linewidth]{./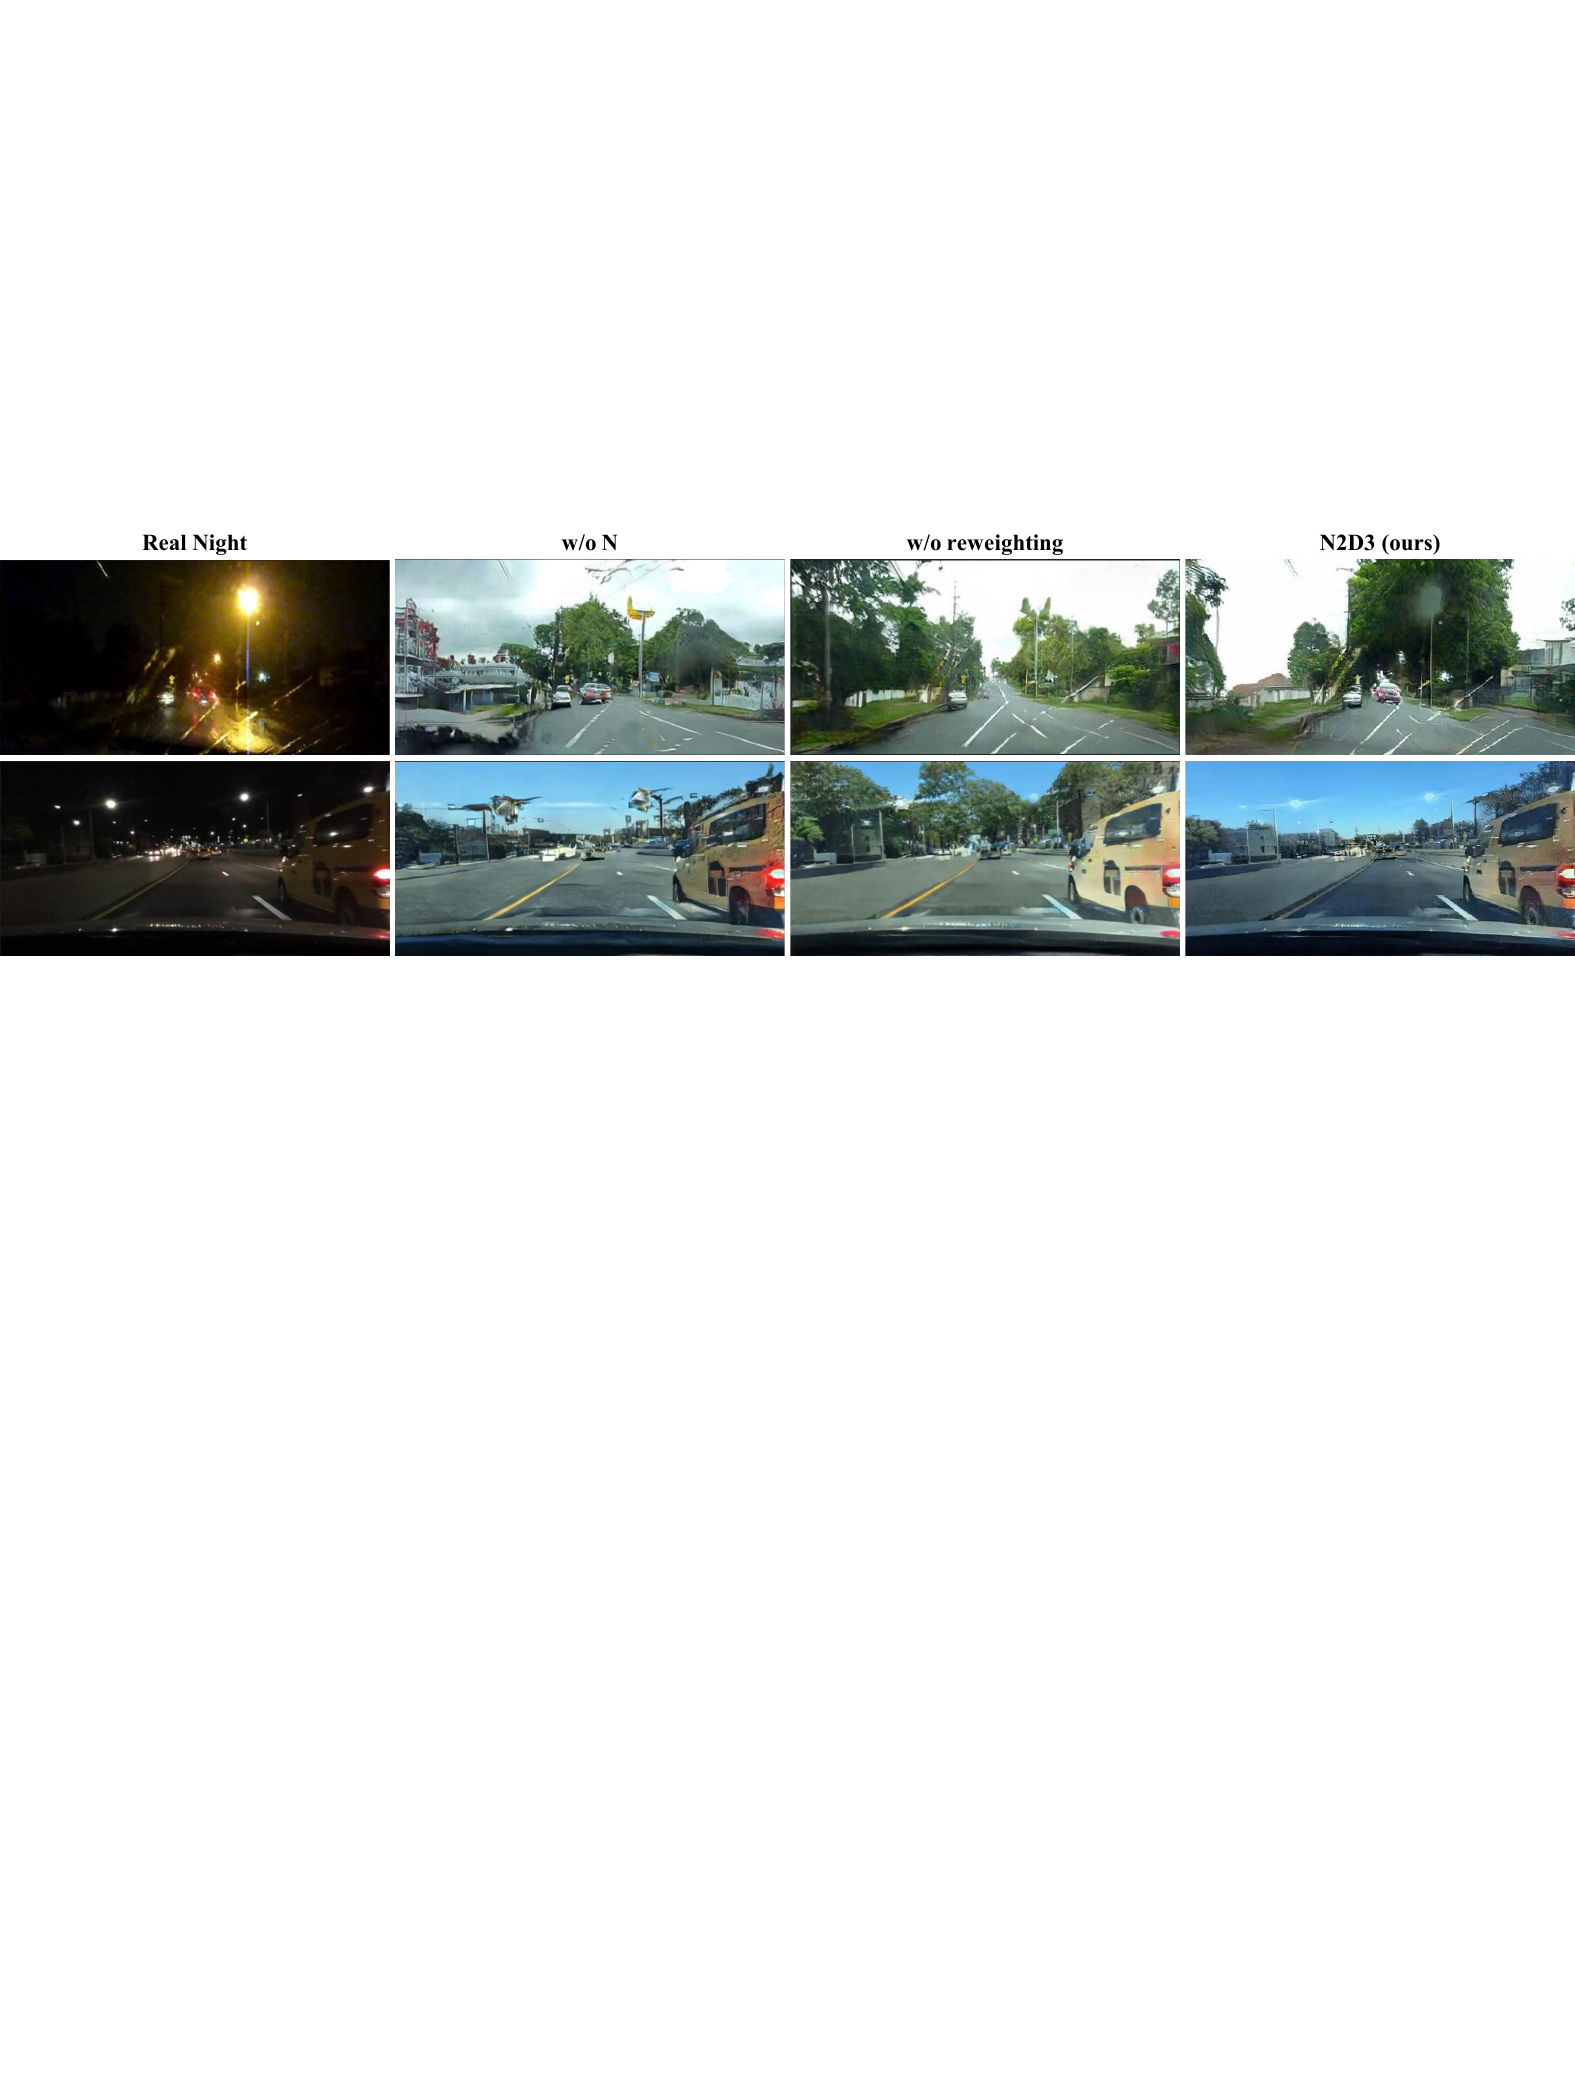} 
\vspace{-0.2cm}
\caption{Qualitative comparison abalation results.}
\vspace{-0.3cm}
\label{fig: abalation results supp}
\end{figure*}

\section{More Visualization Results}\label{sec:4}
\textbf{More Ablation Visualization Results.}
We provide ablation visualization results on both Alderley and BDD100K in \cref{fig: abalation results supp}. The complete method is presented along with ablation studies on the invariant $N$ and without degradation-aware reweighting. All the modules contribute to improving the ability to maintain semantic consistency.

\textbf{More Disentanglement Results.}
We provide additional disentanglement results in \cref{fig: dis results supp}. Our disentanglement methods offer a comprehensive representation of different illumination degradation types in various nighttime scenes.

\textbf{More Qualitative Comparison.}
We present more qualitative comparisons in \cref{fig: alder results supp} and \cref{fig: bdd results supp} alongside other methods.Our method demonstrates visually pleasing results under various nighttime conditions.

\begin{figure*}[htbp]
\centering
\vspace{-0.4cm}
\includegraphics[width=1\linewidth]{./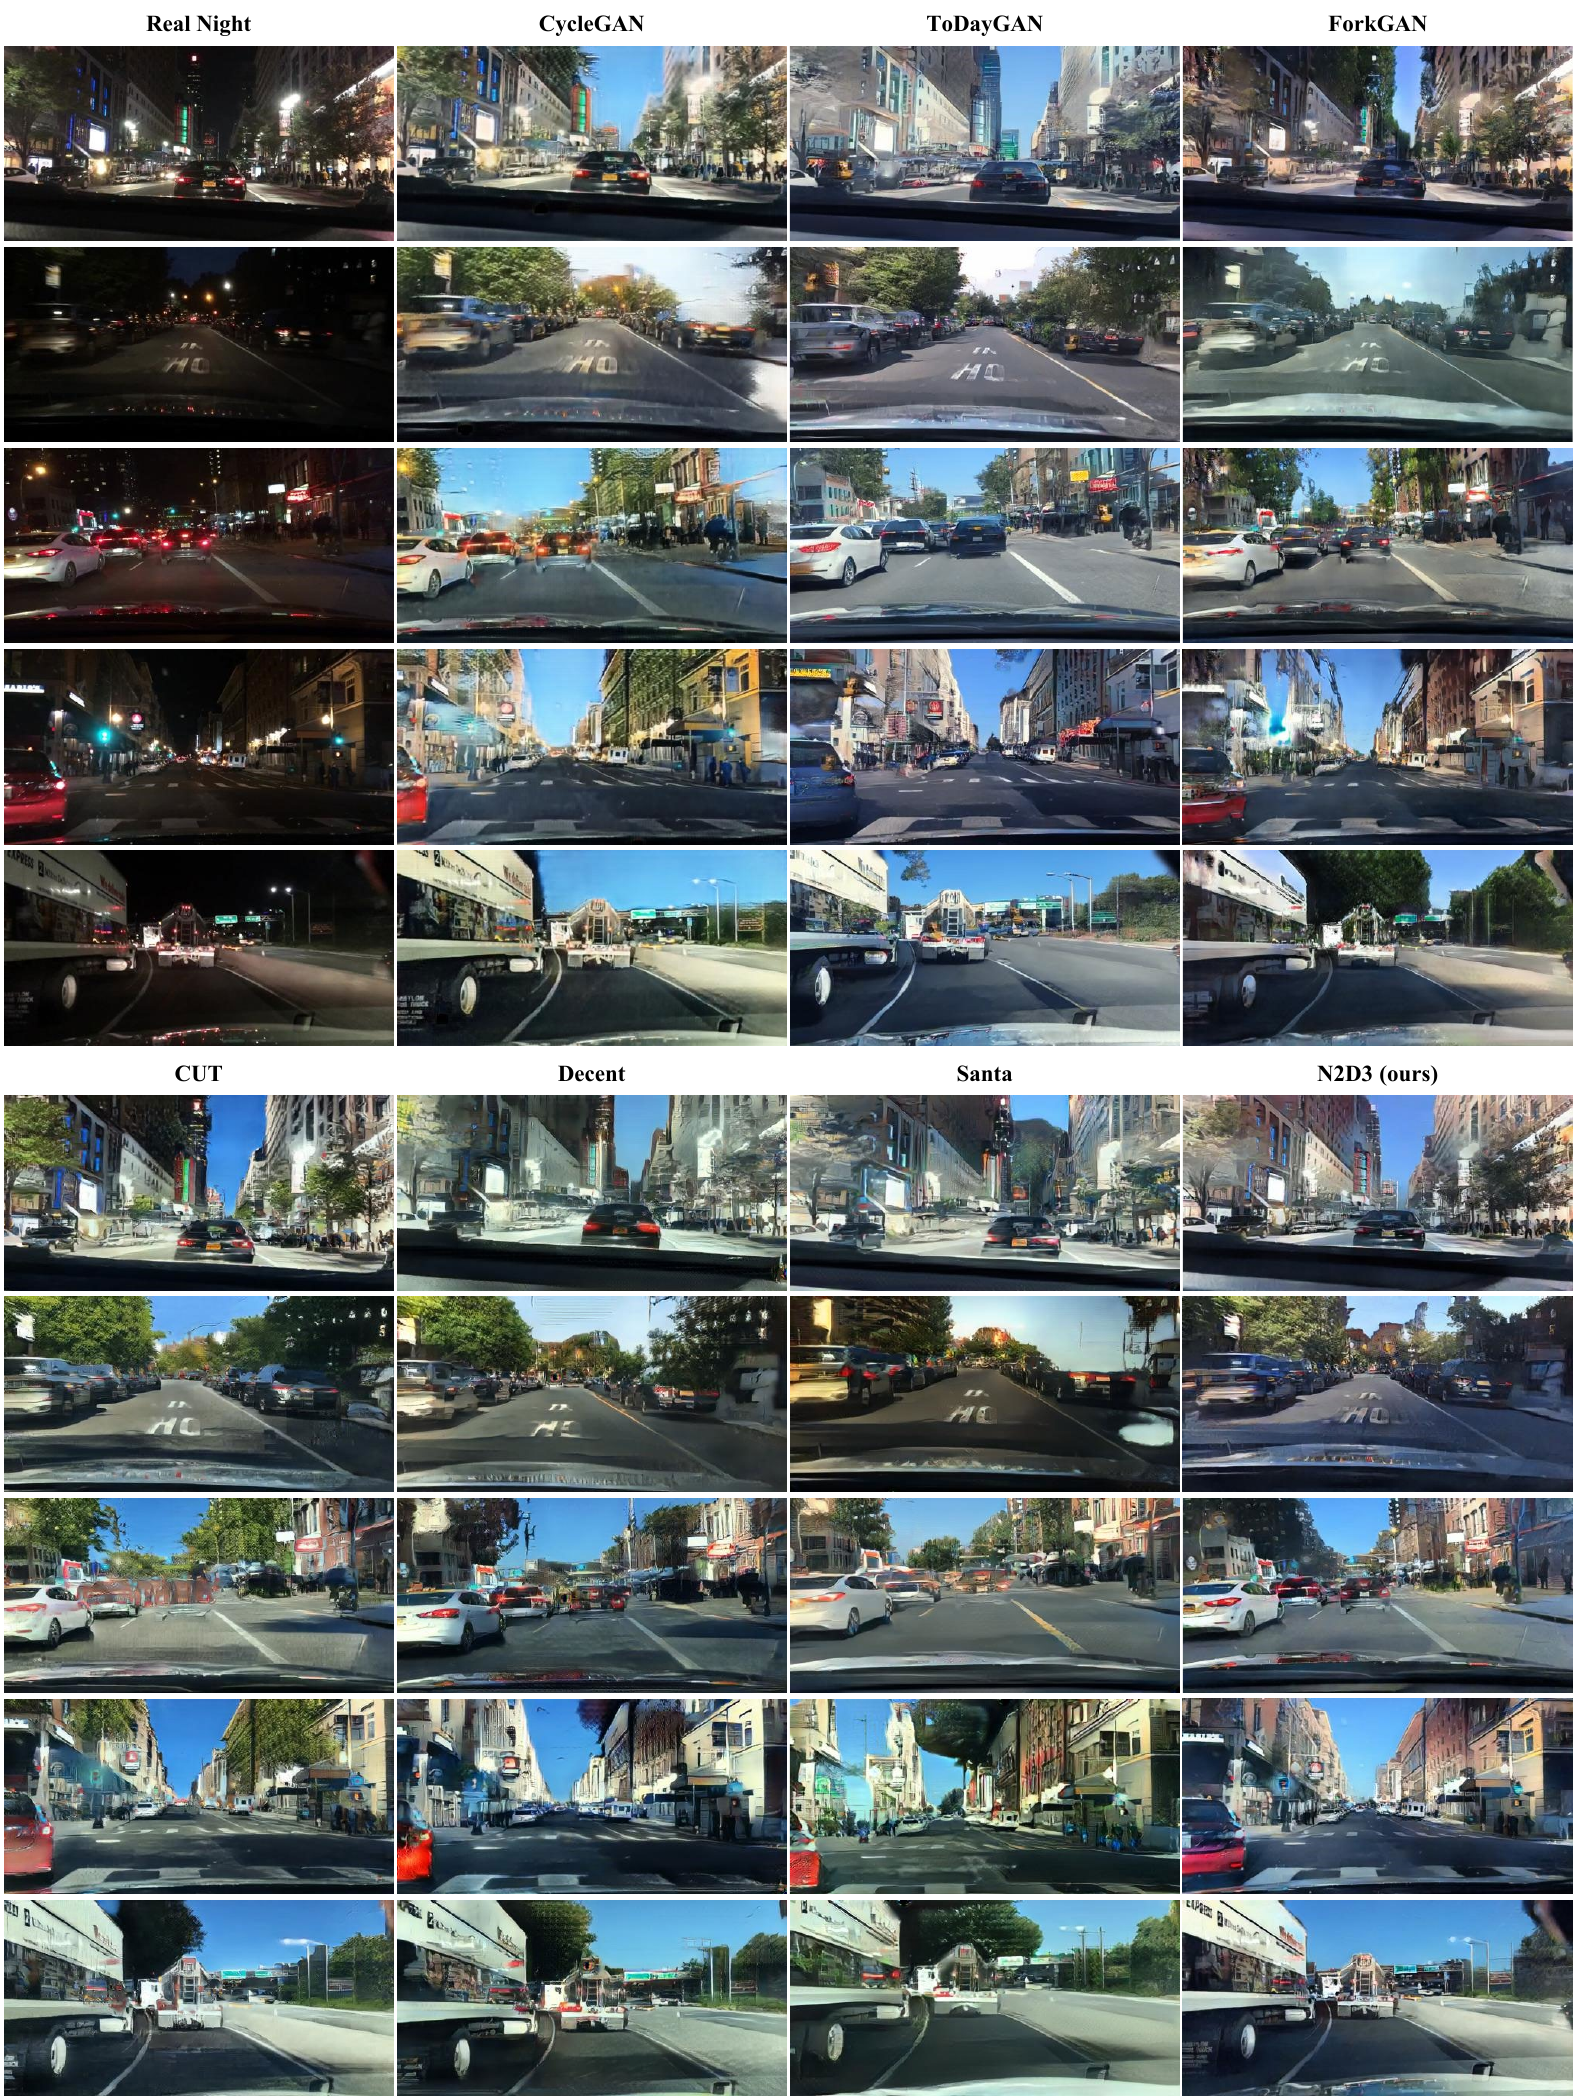}
\vspace{-0.2cm}
\caption{More qualitative comparison results on the BDD100K dataset.}
\vspace{-0.2cm}
\label{fig: bdd results supp}
\end{figure*}

 \begin{figure*}[htbp]
\vspace{-0.4cm}
\includegraphics[width=1\linewidth]{./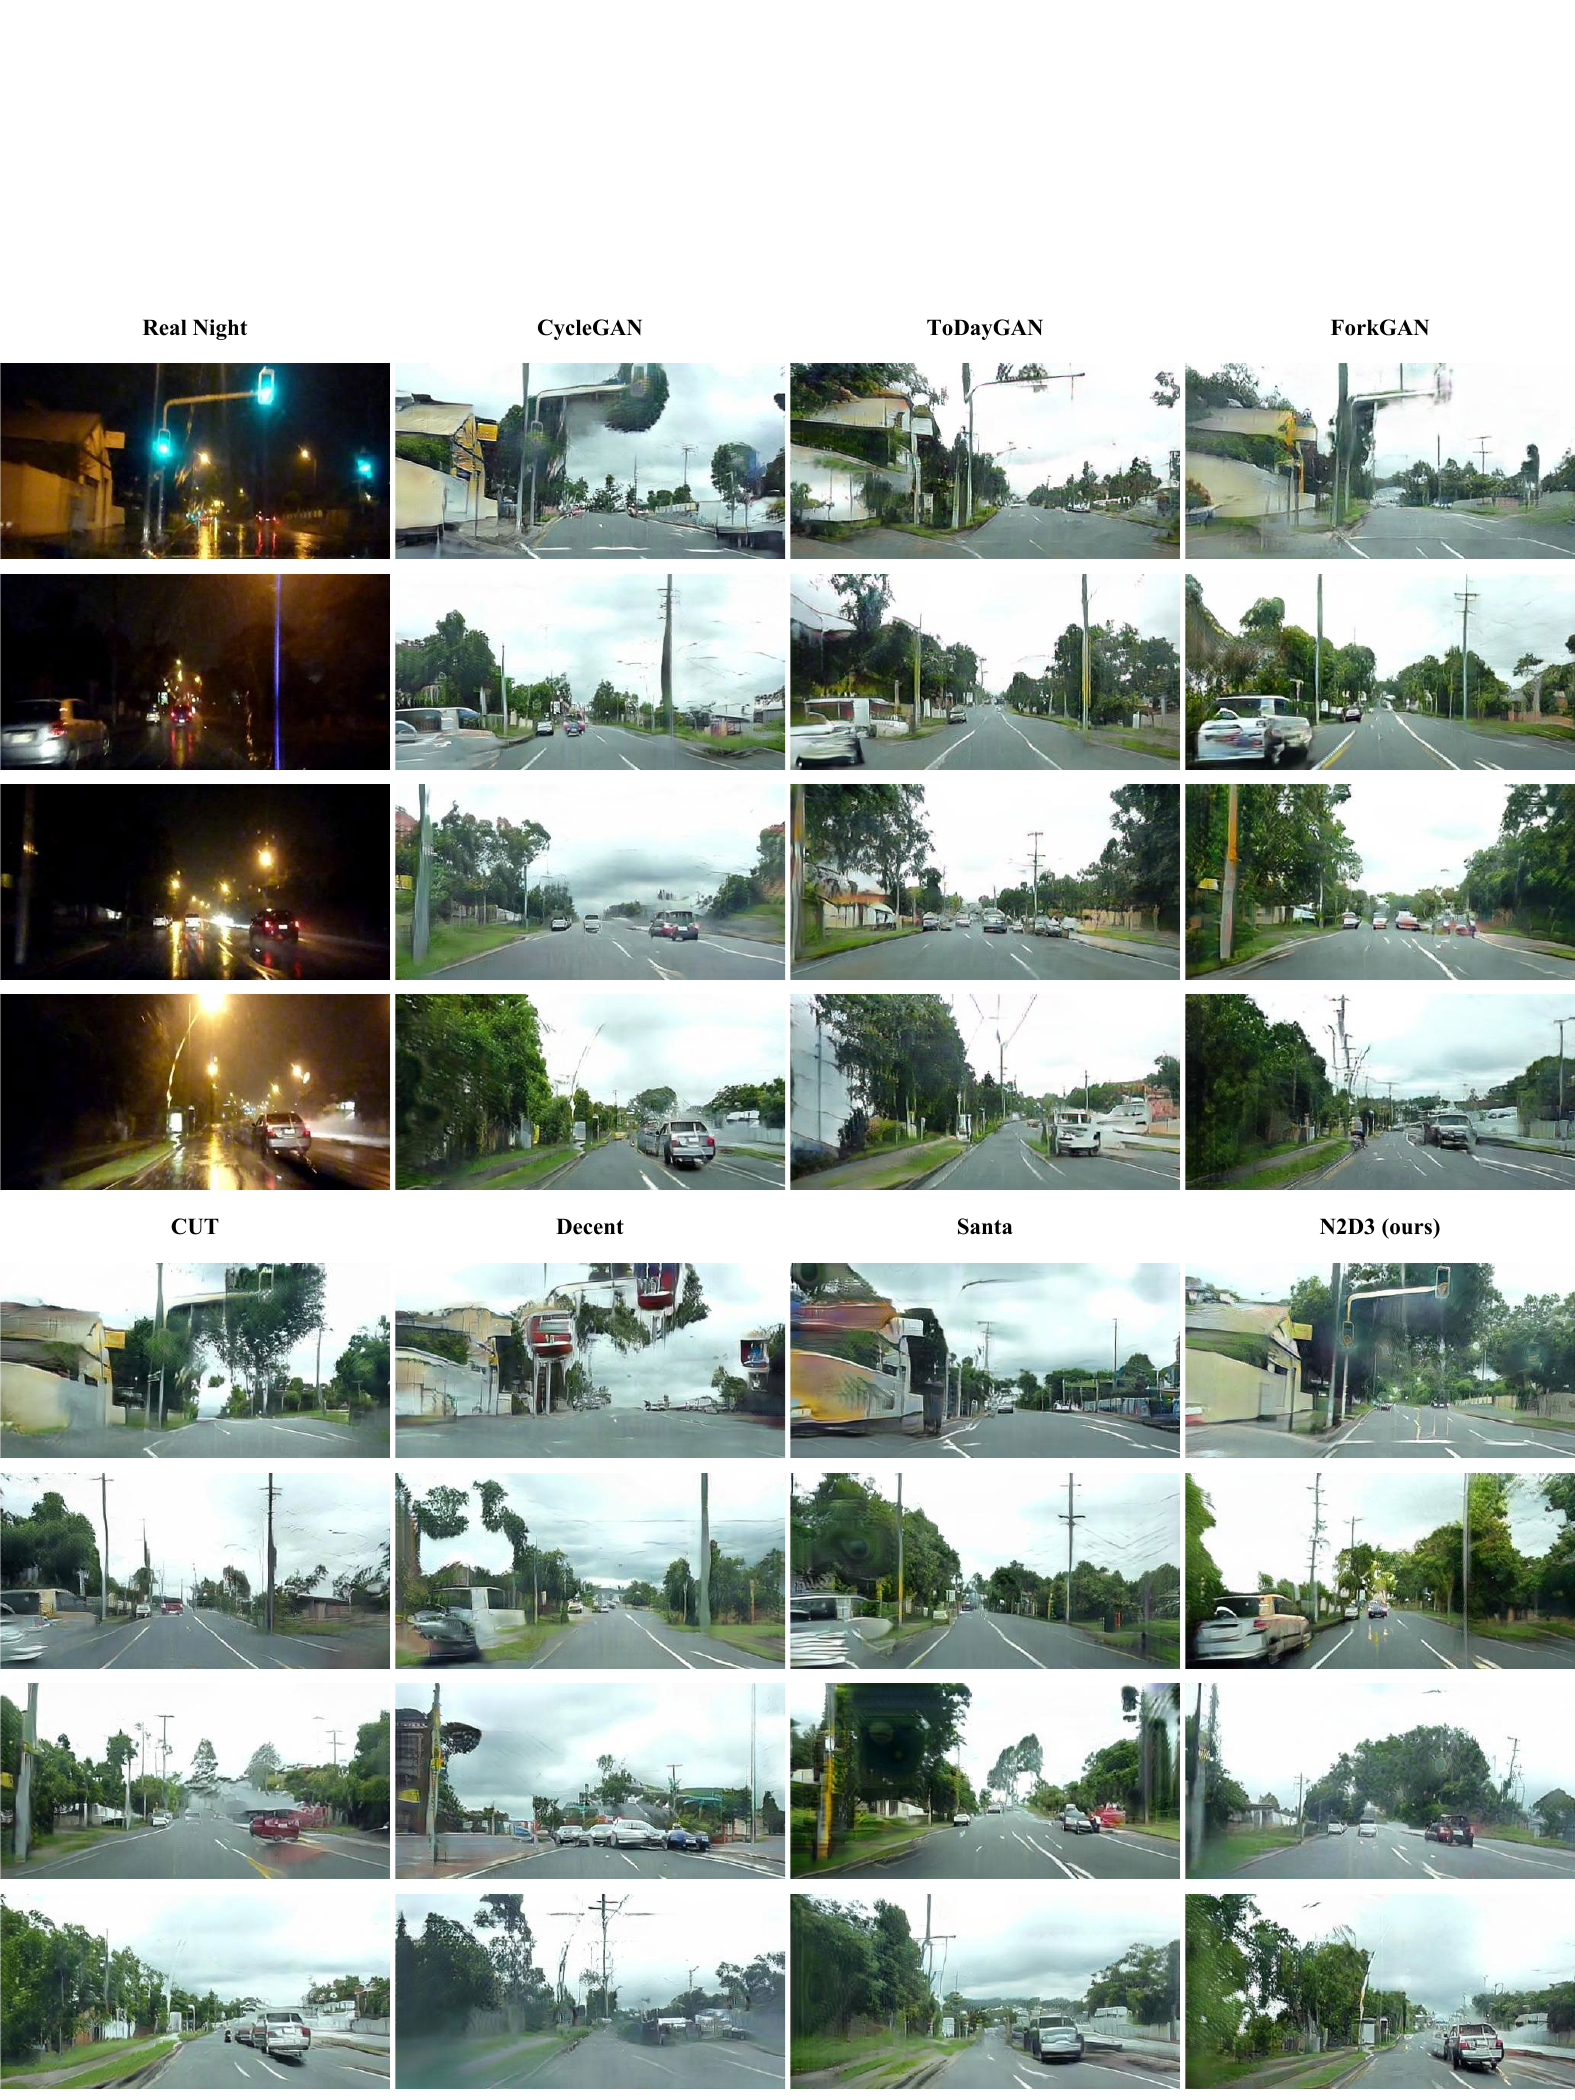} 
\vspace{-0.2cm}
\caption{More qualitative comparison results on the Alderley dataset. }
\vspace{-0.3cm}
\label{fig: alder results supp}
\end{figure*}
